# Supplementary material for: Surface Normal Estimation of Tilted Images via Spatial Rectifier
Source: arXiv:2007.09264 source file (2022-07-14)
Supplement: Supplementary file 1 [file Appendix.tex]

\section{Appendix}
\subsection{Equivalency of surface normal representations}
The unit vector can be decomposed into angle representation as tilt (azimuth) ($\phi$) and slant (polar) ($\theta$) (see Figure~\ref{fig:angle_representation}) as follows:
\begin{equation}
    \mathbf{n} = 
    \begin{bmatrix}
    cos(\theta) cos(\phi) \\
    cos(\theta) sin(\phi) \\ 
    sin(\theta)
    \end{bmatrix} \label{eq:normal_angle_representation}
\end{equation}
% \begin{figure}[ht]
% \begin{center}
% \includegraphics[width=0.4\textwidth]{sections/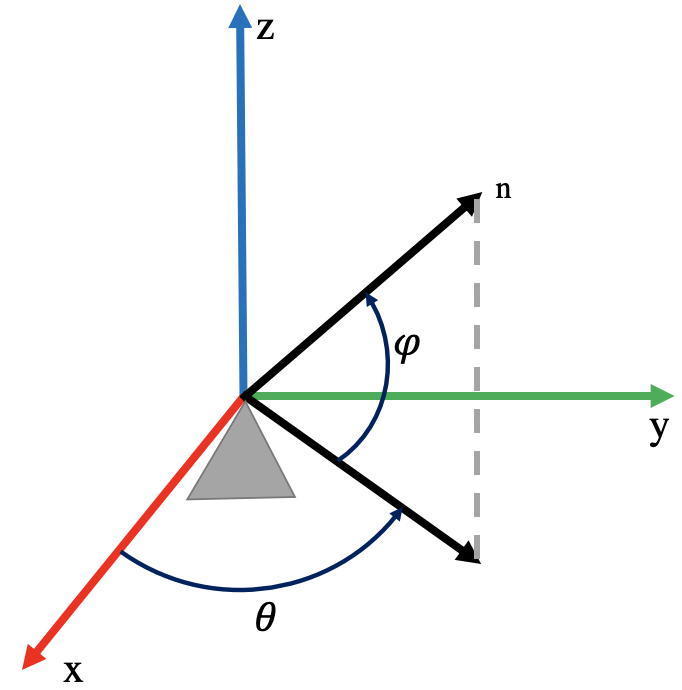} 
% \end{center}
% \caption{Angle representation ($\theta, \phi$) of a unit vector $\mathbf{n}$ in a camera frame of reference}
% \label{fig:angle_representation}
% \end{figure} 
%
The network learns to predict $\widehat\theta, \widehat{\mathbf{z}}$
via supervised-train with ground-truth $\theta, \mathbf{z}$.
Given the surface normal ground-truth $\mathbf{n} = \begin{bmatrix} n_{x} & n_{y} & n_{z}\end{bmatrix}^{T}$ and denote $\xi = (n_{x})^{2} + (n_{y})^{2}$, we compute the supervised ground-truth for the angles prediction as follows:
\begin{align}
    \text{if } \xi < \epsilon:& \begin{cases}
        \mathbf{z} = \mathbf{0} \\
        \theta = \frac{\pi}{2}
    \end{cases} \\
    \text{else }:& \begin{cases}
        \mathbf{z} = \begin{bmatrix} n_{x} \\ n_{y} \end{bmatrix} \\
        \theta = \text{atan2}(n_{z}, \sqrt{\xi})
    \end{cases}
\end{align}
Note that to prevent ambiguity in $\mathbf{z}$, we have enforced it to be exactly $\mathbf{0}$ when $\phi \simeq \frac{\pi}{2}$.
\begin{figure}[ht]
\includegraphics[width=0.4\textwidth]{sections/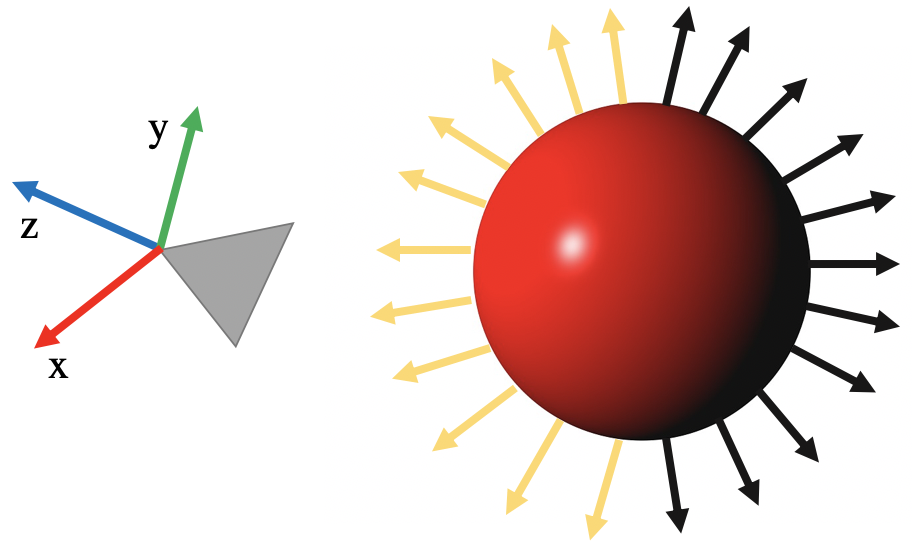} 
\centering
\caption{Visibility of surface normal direction: A camera is looking at a sphere, the yellow surface normal are those that are visible by the camera while the black one are not.}
\label{fig:camera_sphere}
\end{figure}
In addition, notice that the visible parts of the scene are those that have the surface normal vector formed an accute angle with the z-axis of the camera (see Figure~\ref{fig:camera_sphere}).
This would yield an algebraic constraint on the surface normal prediction:
\begin{equation}
    \hat{n}_{z} > 0 \Leftrightarrow \widehat\theta \in [0, \frac{\pi}{2}] 
\end{equation}

\subsection{Proof of Theorem~\ref{theorem:upperbound_on_MAE}}

\begin{proof}
Given $\widehat{\mathbf{n}}$, $\mathbf{n}$ and theirs corresponding slant angles $\widehat\theta$, $\theta$, tilt angles $\widehat\phi$, $\phi$ (see Figure~\ref{fig:camera_sphere}), respectively.
We first show the following result (triangle inequality in angular domain):
\begin{align}
    \min\{|\phi-\hat\phi|, 2\pi- &|\phi-\hat\phi|\} + |\theta-\hat\theta| \geq \delta\label{eq:triangle_ineq_angular_domain} \\
    \Delta\phi + \Delta\theta  \geq \delta \nonumber
\end{align}
where $\delta = cos^{-1}(\hat{\mathbf{n}}^T \mathbf{n})$ is the angular error between these 2 vectors.

To compute the tilt angle error, we first need to project $\widehat{\mathbf{n}}$ and $\mathbf{n}$ on $xy$-plane as $\boldsymbol{\Uppi} \hat{\mathbf{n}}$ and $\boldsymbol{\Uppi} \mathbf{n}$, respectively, where $\boldsymbol{\Uppi}$ is the projection matrix defined as $\boldsymbol{\Uppi} = \begin{bmatrix}1 & 0 & 0\\ 0 & 1 & 0\end{bmatrix}$.
Note that if either $\widehat{\mathbf{n}}$ or $\mathbf{n}$ is orthogonal to $xy$-plane, then $\delta = |\theta - \hat\theta|$, and~\eqref{eq:triangle_ineq_angular_domain} holds trivially.
Therefore, we only focus on the case where neither $\widehat{\mathbf{n}}$ nor $\mathbf{n}$ is orthogonal to $xy$-plane, or equivalently, $||\boldsymbol{\Uppi}\widehat{\mathbf{n}}||$ and $||\boldsymbol{\Uppi} \mathbf{n}||$ are strictly positive.
The tilt error $\Delta\phi$, finally, can then be computed as:
\begin{align*}
    \Delta \phi &= \min\{|\phi-\hat\phi|, 2\pi- |\phi-\hat\phi|\} \\
    &= cos^{-1}(\frac{(\boldsymbol{\Uppi} \hat{\mathbf{n}})^T (\boldsymbol{\Uppi} \mathbf{n} )}{\| \boldsymbol{\Uppi} \hat{\mathbf{n}} \| \| \boldsymbol{\Uppi} \mathbf{n}\|})
\end{align*}
The slant angles $\hat\theta$ and $\theta$ can be subsequently computed as:
\begin{align}
    \hat\theta &= \frac{\pi}{2} - cos^{-1}(||\boldsymbol{\Uppi}\widehat{\mathbf{n}}||) \\
    \theta &= \frac{\pi}{2} - cos^{-1}(||\boldsymbol{\Uppi}{\mathbf{n}}||)
\end{align}
Finally, the slant error $\Delta \theta$ can be computed as:
\begin{align*}
\Delta \theta &= |cos^{-1}(\| \boldsymbol{\Uppi} \hat{\mathbf{n}} \|) -  cos^{-1}(\| \boldsymbol{\Uppi} \mathbf{n}  \|) | 
\end{align*}
Based on definitions we have the following identities:
\begin{align*}
cos(\delta) = \hat{\mathbf{n}}^T \mathbf{n} \textnormal{ and }
cos(\Delta \phi) = \frac{(\boldsymbol\Uppi \hat{\mathbf{n}})^T (\boldsymbol\Uppi \mathbf{n})}{\| \boldsymbol{\Uppi} \hat{\mathbf{n}} \| \cdot \| \boldsymbol{\Uppi} \mathbf{n} \|}
\end{align*}
\begin{equation*}
\begin{split}
cos(\Delta \theta) & = cos(cos^{-1}(\| \boldsymbol{\Uppi} \hat{\mathbf{n}} \|) - cos^{-1}(\| \boldsymbol{\Uppi} \mathbf{n}) \|) \\
 & = \| \boldsymbol{\Uppi} \hat{\mathbf{n}} \| \cdot \| \boldsymbol{\Uppi} \mathbf{n} \| + (\mathbf{n} - \boldsymbol{\Uppi}\mathbf{n})^T(\hat{\mathbf{n}} - \boldsymbol{\Uppi}\hat{\mathbf{n}})
\end{split}
\end{equation*}
Furthermore, note that from $\delta, \Delta \phi \in [0, \pi]$ and $\Delta \theta \in [0, \frac{\pi}{2}]$, we have:
\begin{align}
    sin(\Delta \phi), \ sin(\Delta \theta) \textnormal{ and } cos(\Delta \theta) \geq 0 \label{eq:sttsphicphi_geq_0}
\end{align}
We consider 2 cases: 

Case 1: $\Delta \phi + \Delta \theta > \pi \nonumber$ then $\Delta \phi + \Delta \theta > \pi \geq \delta$ hence~\eqref{eq:triangle_ineq_angular_domain} holds trivially.

Case 2: $\Delta \phi + \Delta \theta \leq \pi$. From~\eqref{eq:sttsphicphi_geq_0}, we have:
\begin{align}
\begin{split}
cos(\Delta \phi + \Delta \theta) = cos(\Delta \phi)&cos(\Delta \theta) \nonumber \\ & -sin(\Delta \phi)sin(\Delta \theta)
\end{split} \nonumber \\
\leq cos(\Delta \phi)&cos(\Delta \theta) \label{eq:cos_ttplus_phi}
\end{align}
where~\eqref{eq:cos_ttplus_phi} is obtained due to~\eqref{eq:sttsphicphi_geq_0}. Next we examine:
\begin{align}
cos(&\Delta \phi)cos(\Delta \theta) \nonumber \\ & = (\boldsymbol\Uppi \hat{\mathbf{n}})^T (\boldsymbol\Uppi \mathbf{n}) \nonumber \\  & \ \ \ \ \ \ + cos(\Delta \phi) (\mathbf{n}  - \boldsymbol{\Uppi}\mathbf{n} )^T(\hat{\mathbf{n}} - \boldsymbol{\Uppi}\hat{\mathbf{n}}) \nonumber \\
& \leq (\boldsymbol\Uppi \hat{\mathbf{n}})^T (\boldsymbol\Uppi \mathbf{n} ) + (\hat{\mathbf{n}} - \boldsymbol{\Uppi}\hat{\mathbf{n}})^T(\mathbf{n}  - \boldsymbol{\Uppi}\mathbf{n} ) \label{eq:costt_leq_1} \\
& = \hat{\mathbf{n}}^T \mathbf{n}  = cos(\delta) \label{eq:dotproduct}
\end{align}
where~\eqref{eq:costt_leq_1} is obtained due to $cos(\Delta \phi) \leq 1$ and $(\hat{\mathbf{n}} - \boldsymbol{\Uppi}\hat{\mathbf{n}})^T(\mathbf{n}  - \boldsymbol{\Uppi}\mathbf{n} ) \geq 0$, and~\eqref{eq:dotproduct} is obtained by noticing that $ ((\mathbf{x} - \boldsymbol{\Uppi} \mathbf{x})^T (\boldsymbol{\Uppi} \mathbf{y}) = 0 \ \forall \mathbf{x}, \mathbf{y} \in \mathbb{R}^3)$. 
From~\eqref{eq:cos_ttplus_phi} and case 2 condition, we have:
\begin{align*}
& cos(\Delta \phi + \Delta \theta) \leq cos(\delta) \\
\implies & \Delta \phi + \Delta \theta \geq \delta    
\end{align*}
The equality happens when $cos(\Delta \theta) = 1$ or $\Delta\theta = 0$.
Given the triangle inequality in angular domain~\eqref{eq:triangle_ineq_angular_domain}, it is straightforward to add up each component of the loss function $\mathcal{L}_{\boldsymbol{\Theta}}$ and the mean of absolute angular error $\mathcal{L}_{\delta}$ and obtained Theorem~\ref{theorem:upperbound_on_MAE}.
\end{proof}
